# Supplementary material for: Dynamical Low-Rank Ensemble Kalman filter for State/Parameter estimation
Source: arXiv:2602.06614 source file (2026-10-08)
Supplement: Supplementary file 1 [file appendix.tex]

\section{Appendix}

As in~\cite{DynamicalLoTrigo2025}, we begin by presenting the construction of the DLR filtering process in the mean-field sense, and motivate the formulation of the practical particularised versions based on them. 
Focussing on the \vkbp, the dynamics for the state may be rewritten as 
\begin{align*}
	\rd \Xcal_t &= (f(\Xcal_t, \theta_t) - P_t S \Xcal_t) \rd t 
	%+ [\Soh, - P_t H^{\top} \Gmoh] [\rd \Wcal_t, \rd \Vcal_t]^{\top} 
	- P_t H^{\top} \Gmoh \rd \Vcal_t
	+ P_{t} H^{\top} \Gamma^{-1} \rd \Zcal_t 
		\\
		    &=  a \rd t + b \rd \Vcal_t + c \rd \Zcal_t,
		    %&=  a \rd t + b \rd \overline{\Wcal}_t + c\rd \Zcal_t,
\end{align*}
where $S = H^{\top} \Gamma^{-1} H$. 
Anticipating the developments below, the following quantities will be of interest.
\begin{align*}
	\E[a \st \Acal_{\Zcal_t}] &= \E [ f(\Xcal_t, \theta_t) \st \Acal_{\Zcal_t}] - P_t S \E[\Xcal_t \st \Acal_{\Zcal_t}], &
        a^{\star} &= f^{\star}(\Xcal_t, \theta_t) - P_t S \Xcal_t^{\star}, 
		     \\
	\E[c \st \Acal_{\Zcal_t}] &= P_t H^{\top} \Gamma^{-1}, 
                  & c^{\star}& = 0,
\end{align*}
With that, following the approach in~\cite{DynamicalLoTrigo2025}, the mean-separated \dlr-\vkbp~equations become
\begin{align*}
	\md U_t^0 &= \E [ f(\Xcal_t, \theta_t) \st \Acal_{\Zcal_t}] \rd t + P_t H^{\top} \Gamma^{-1} (\rd \Zcal_t - H U^0_t \rd t),  \\
	\md \bU_t &= P^{\perp}_{\bU_t} \E[ f^{\star}(\Xcal_t, \theta_t) (\bY_t M_{\bY_t}^{-1}) \st \Acal_{\Zcal_t}]  \md t ,
        %- P_t H^{\top} \Gamma^{-1} \Xcal_t^{\star} 
        \\
	\md \bY_t^{\top} &= \bU_t^{\top} f^{\star}(\Xcal_t, \theta_t) \md t 
	%+ \bU_t^{\top} \Soh \rd \Wcal_t 
	- \bU_t^{\top} P_{t} H^{\top} \Gamma^{-1}( H \Xcal_t^{\star} + \Goh \md \Vcal_t ), 
\end{align*}
where $M_{\bY_t} = \E[Y_t^i Y_t^j \st \Acal_{\Zcal_t}]$ is the (continuous) Gram matrix.
